# Supplementary material for: Differentiable Programming: Efficient Smoothing of Control-Flow-Induced Discontinuities
Source: arXiv:2305.06692 source file (2023-05-11)
Supplement: Supplementary file 1 [file appendix.tex]

%\section{Optmization on Smoothed Crescent Function}
